# Supplementary material for: Coexistence of two types of short-range order in SiGeSn medium-entropy alloys
Source: arXiv:2201.08256 source file (2022-01-20)
Supplement: Supplementary file 1 [file Supp_Info.pdf]

# Supporting Information: Coexistence of two types of short-range order in SiGeSn medium-entropy alloys

Xiaochen Jin, Shunda Chen, and Tianshu Li*

*Department of Civil and Environmental Engineering, George Washington University, Washington, DC 20052*

E-mail: tsli@gwu.edu

Phone: +1 (202) 994-3809. Fax: +1 (202) 994-0127

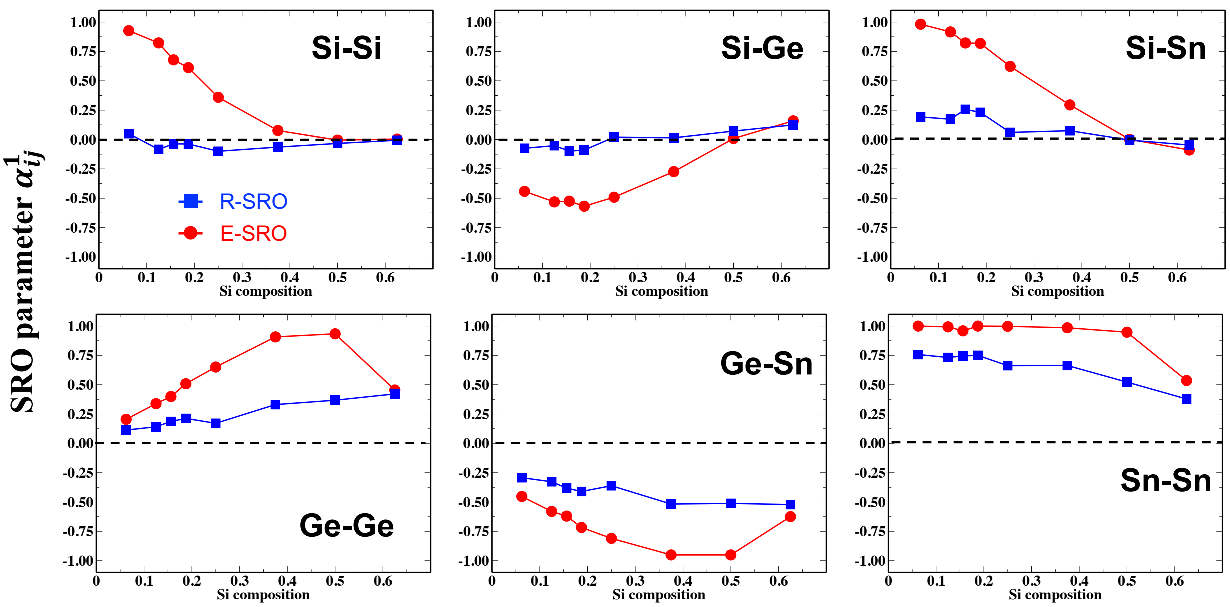


Figure S1: Variation of the first-nearest neighbor SRO parameters $\alpha_{ij}^1$ for all six pairs in $Si_xGe_{0.75-x}Sn_{0.25}$ with Si composition $x$ for R-SRO (blue) and E-SRO (red)

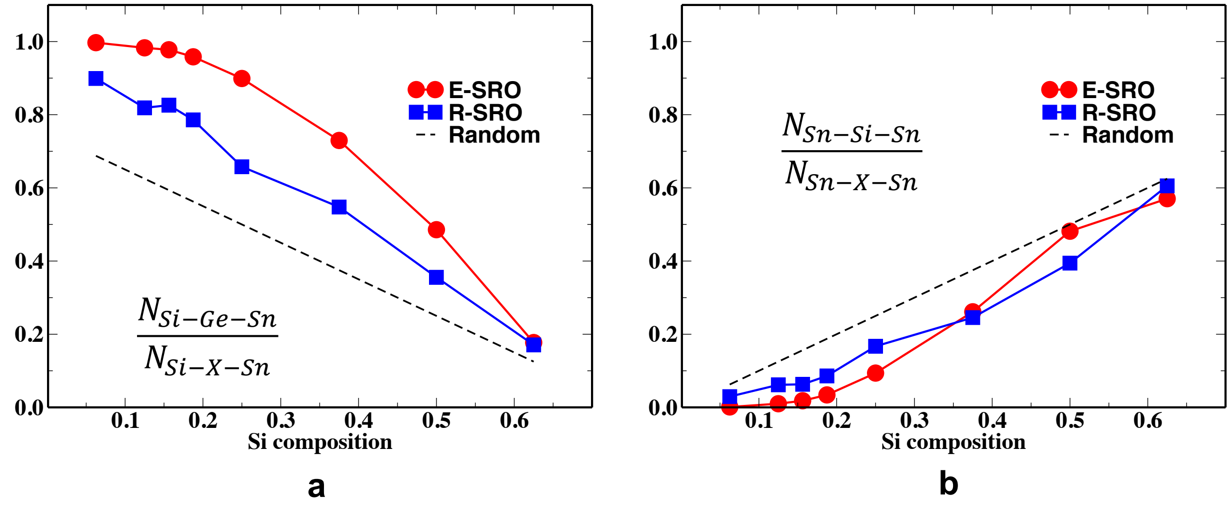


Figure S2: Variation of (**a**) the fraction of Si-Ge-Sn over all possible Si-Sn second-nearest neighbors, namely, Si-X-Sn, where X can be Si, Ge, or Sn, and (**b**) the fraction of Sn-Si-Sn over all possible Sn-Sn second-nearest neighbors, with Si composition $x$ in $Si_xGe_{0.75-x}Sn_{0.25}$.

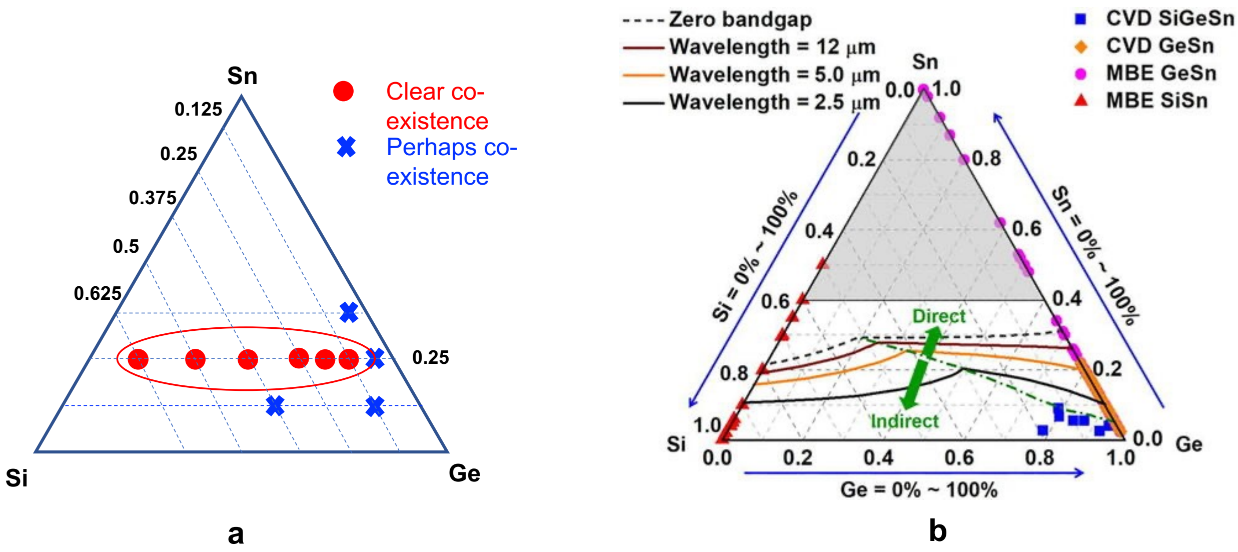


Figure S3: (**a**) Explored compositions of SiGeSn alloy exhibited in Si-Ge-Sn ternary phase space. The compositions that clearly display the co-existence of R-SRO and E-SRO are marked as red dots, whereas those that exhibit signs of but not explicit co-existence in MC samplings are marked as blue cross. These compositions are aligned with (**b**) the published composition diagram showing the predicted constant bandgap contours and indirect-to-direct bandgap partitions (from Ref.[S1]). Particularly, the composition domain where co-existence is identified significantly overlaps the projected composition line of indirect-to-direct transition and the contour lines for mid-infrared applications.

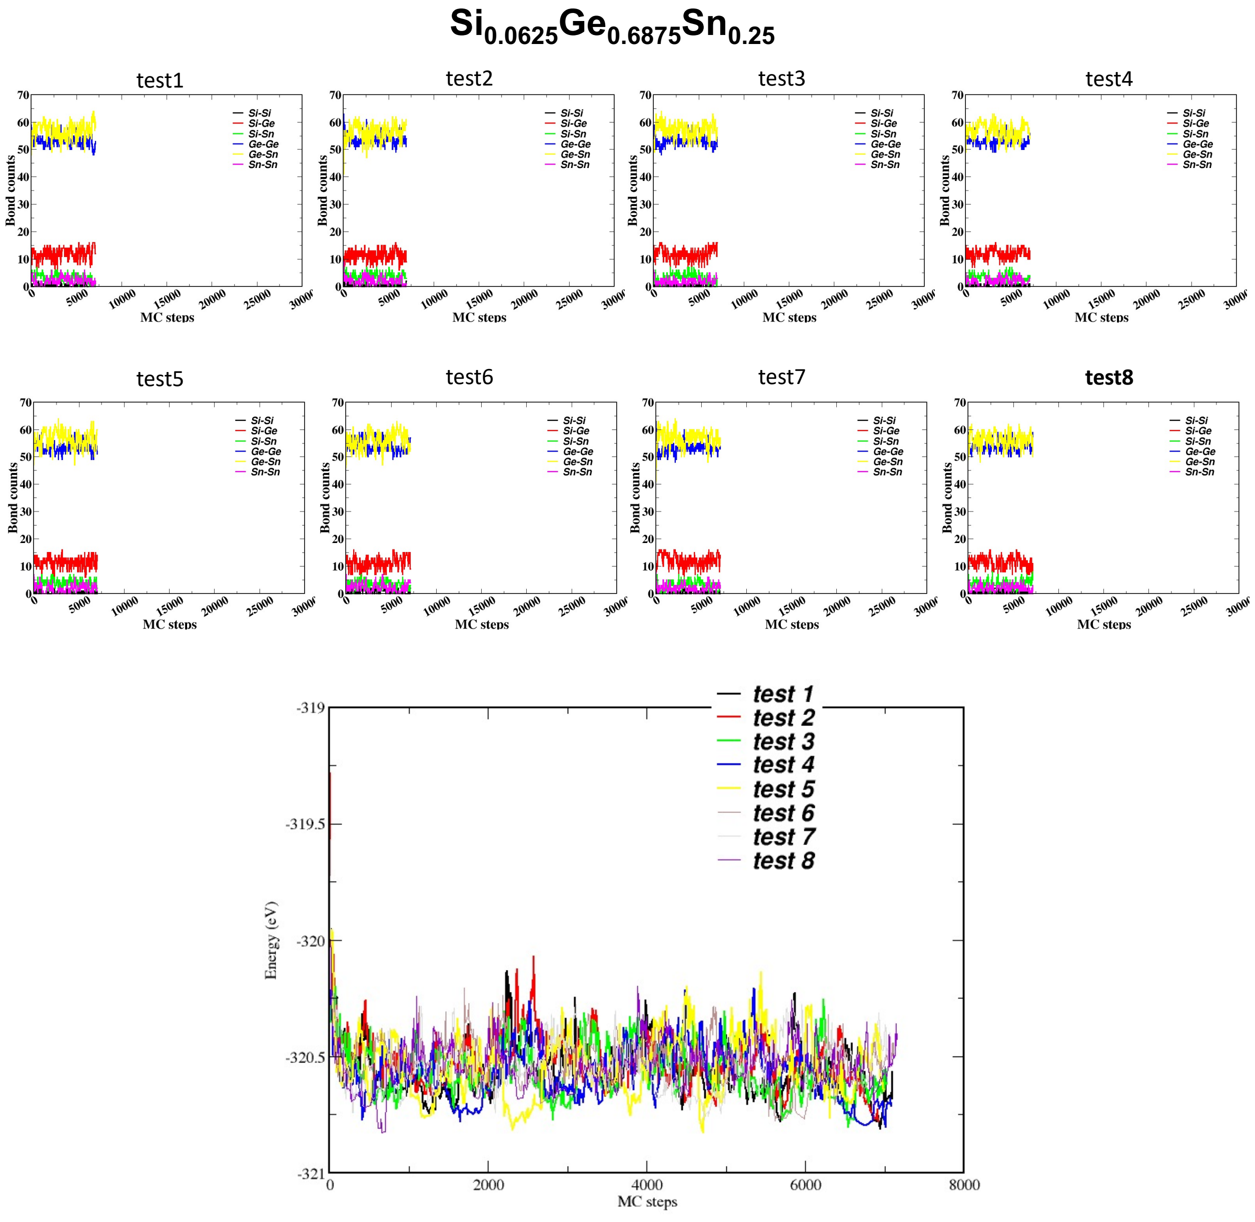


Figure S4: Variation of energy and bonds in MC/DFT sampling for $Si_{0.0625}Ge_{0.6875}Sn_{0.25}$

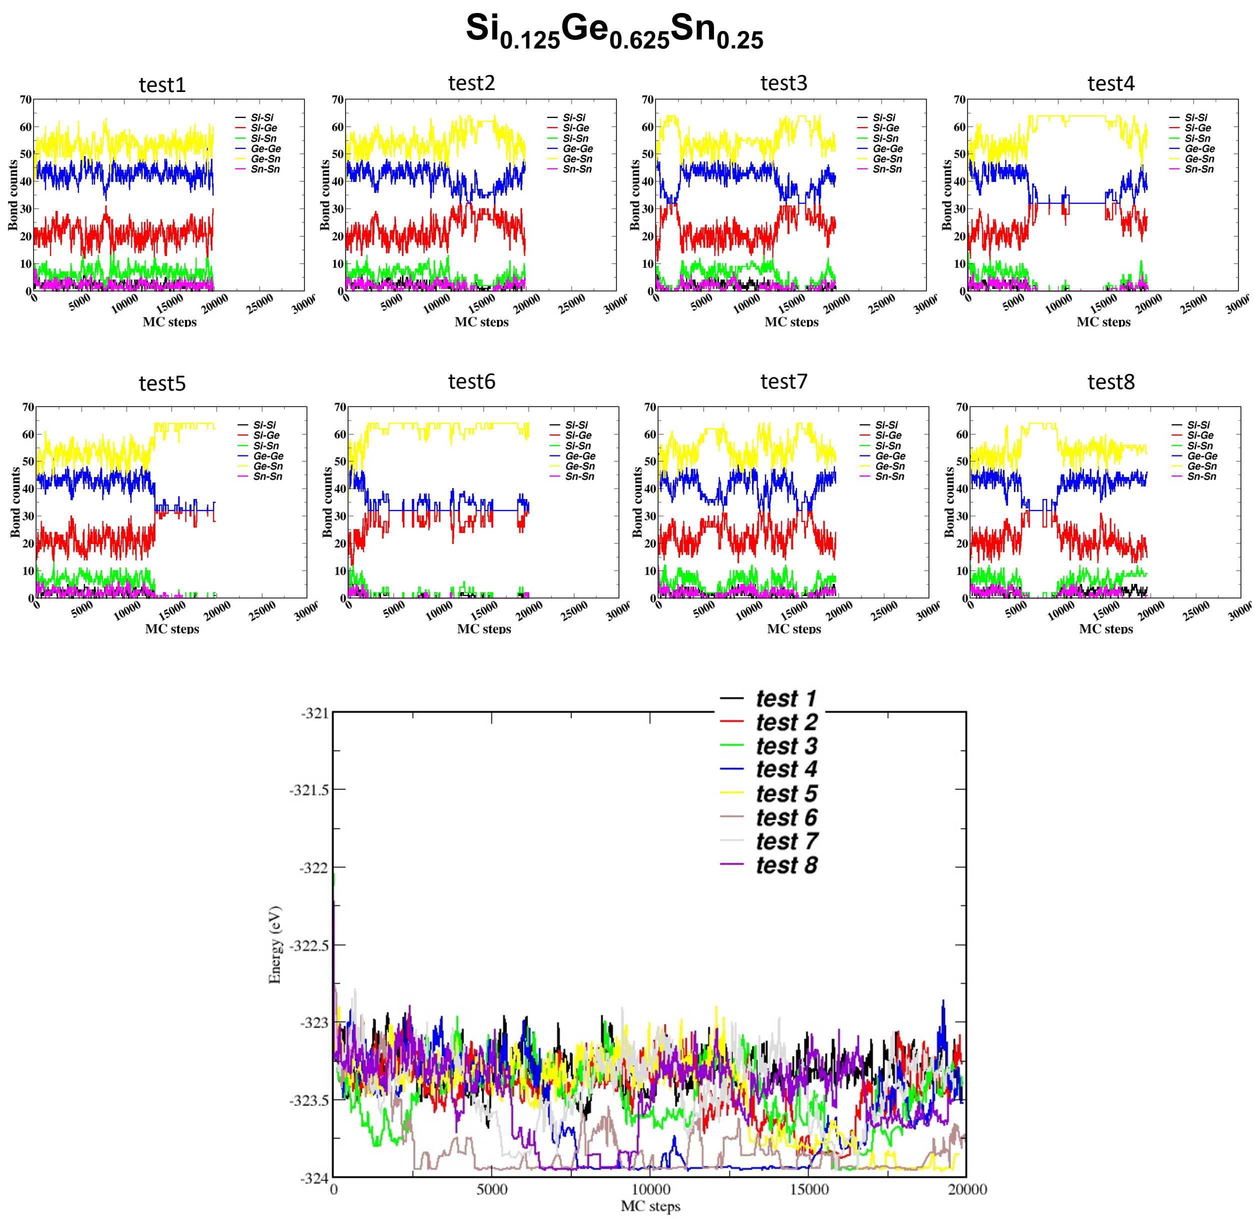


Figure S5: Variation of energy and bonds in MC/DFT sampling for $Si_{0.125}Ge_{0.625}Sn_{0.25}$

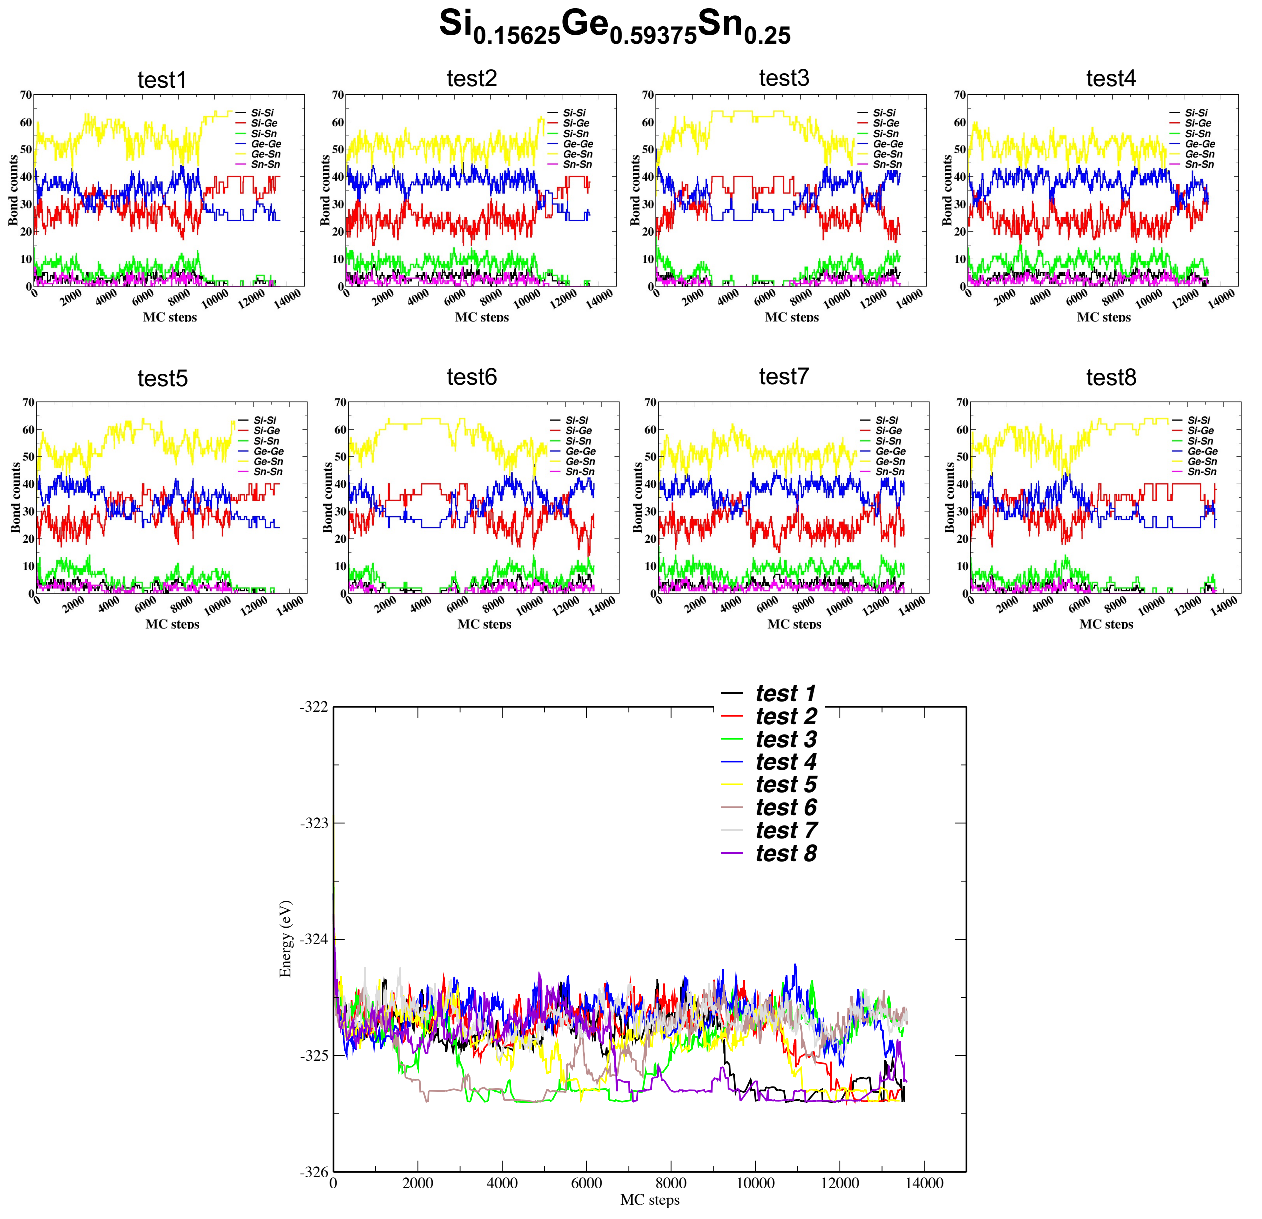


Figure S6: Variation of energy and bonds in MC/DFT sampling for $Si_{0.15625}Ge_{0.59375}Sn_{0.25}$

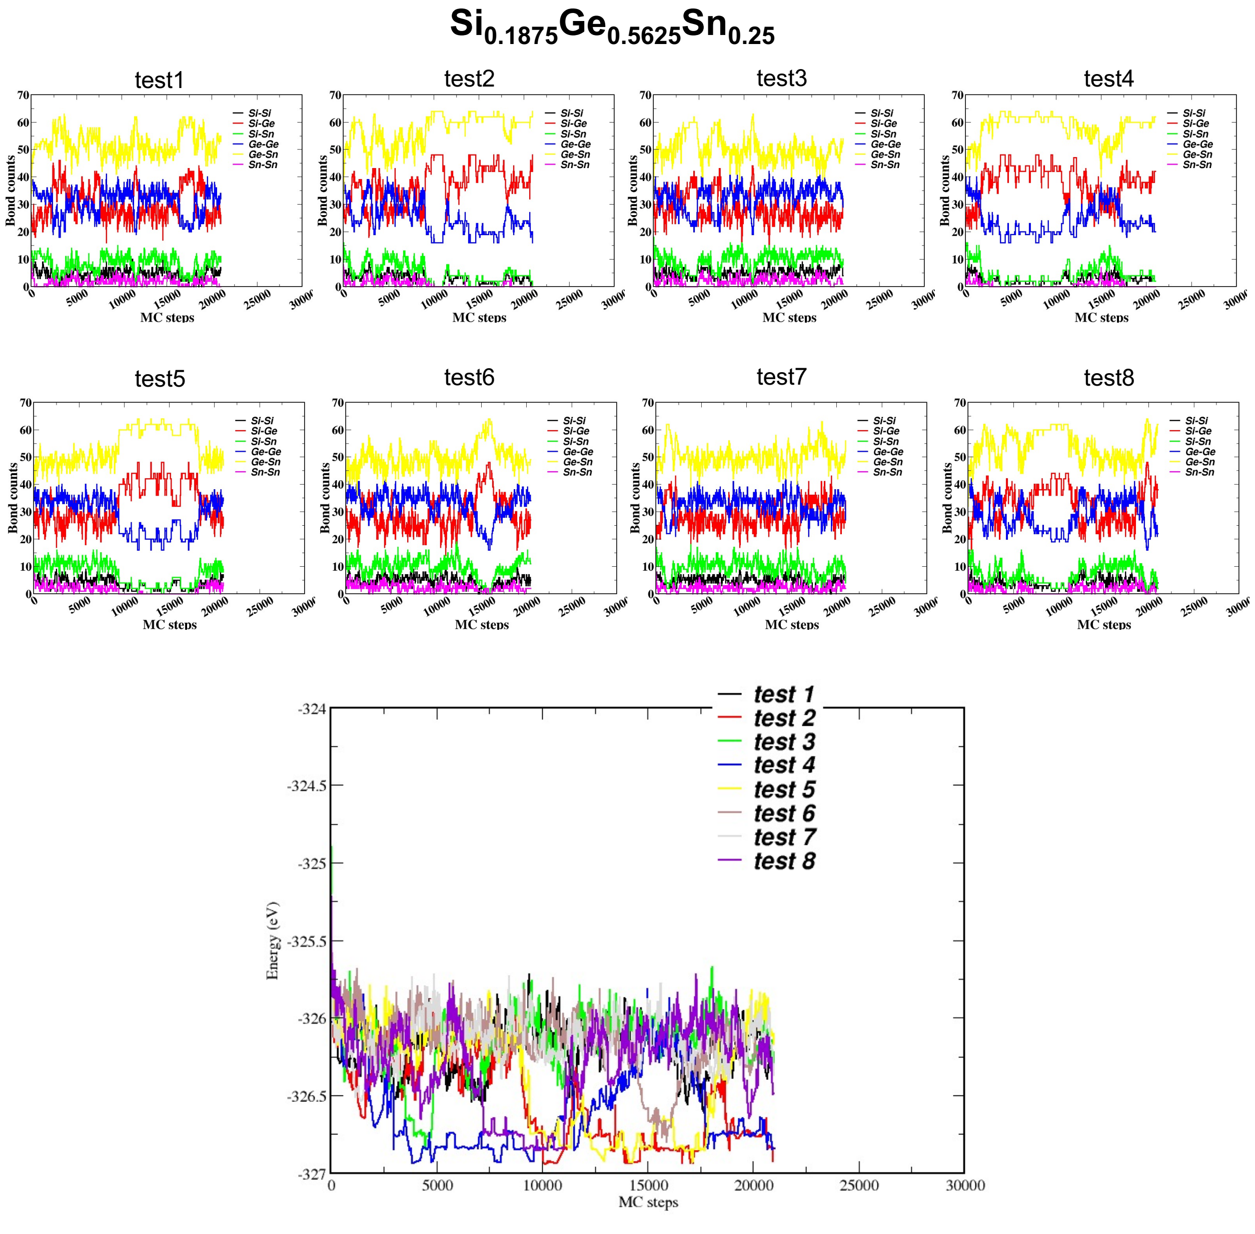


Figure S7: Variation of energy and bonds in MC/DFT sampling for $Si_{0.1875}Ge_{0.5675}Sn_{0.25}$

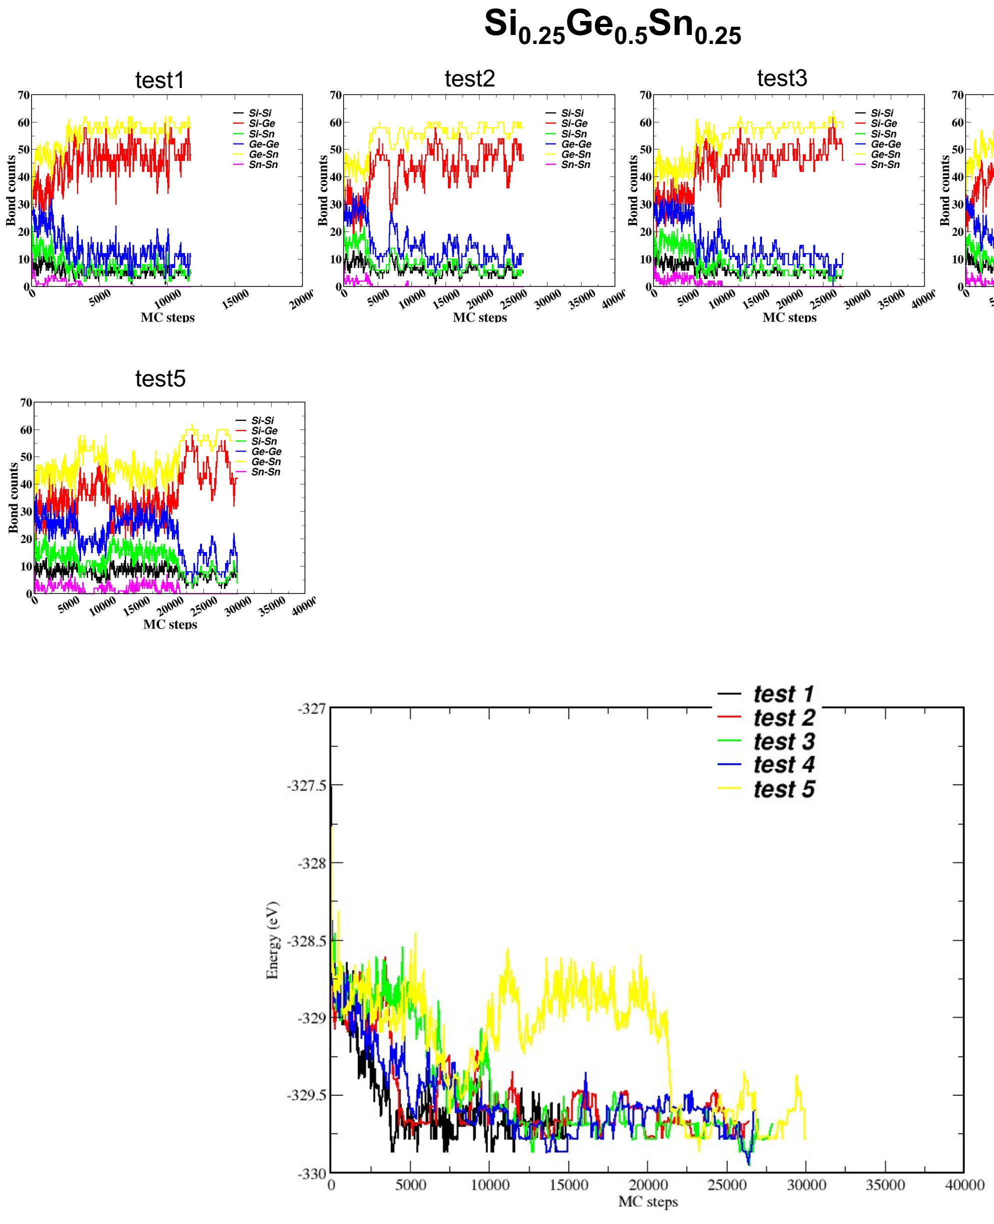


Figure S8: Variation of energy and bonds in MC/DFT sampling for $Si_{0.25}Ge_{0.5}Sn_{0.25}$

## $Si_{0.375}Ge_{0.375}Sn_{0.25}$

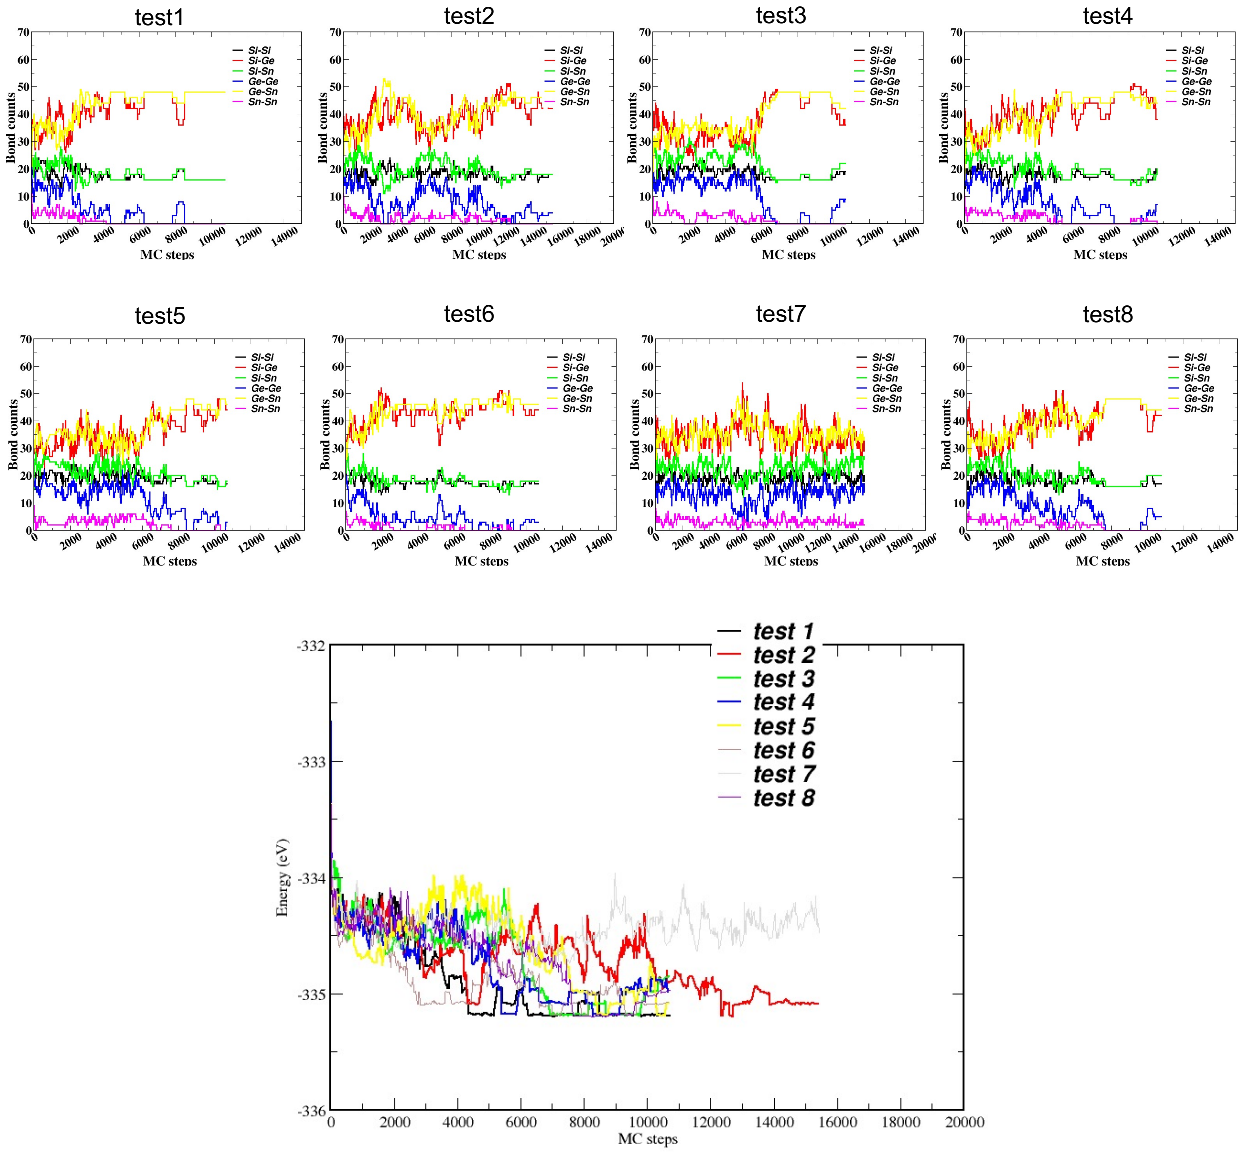


Figure S9: Variation of energy and bonds in MC/DFT sampling for $Si_{0.375}Ge_{0.375}Sn_{0.25}$

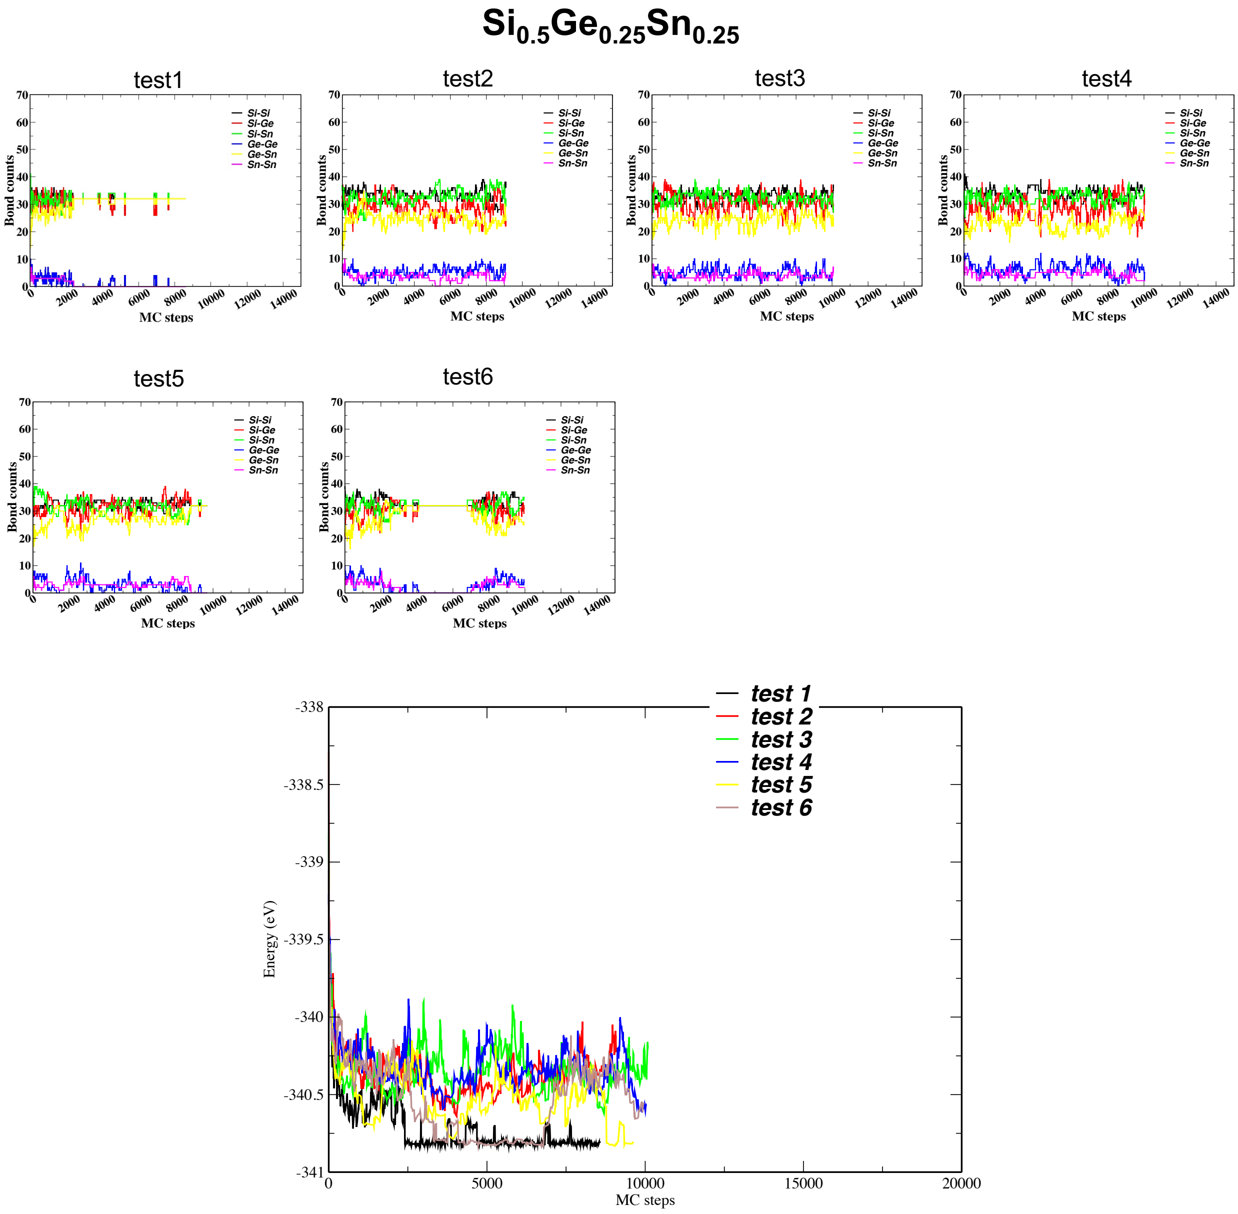


Figure S10: Variation of energy and bonds in MC/DFT sampling for $Si_{0.5}Ge_{0.25}Sn_{0.25}$

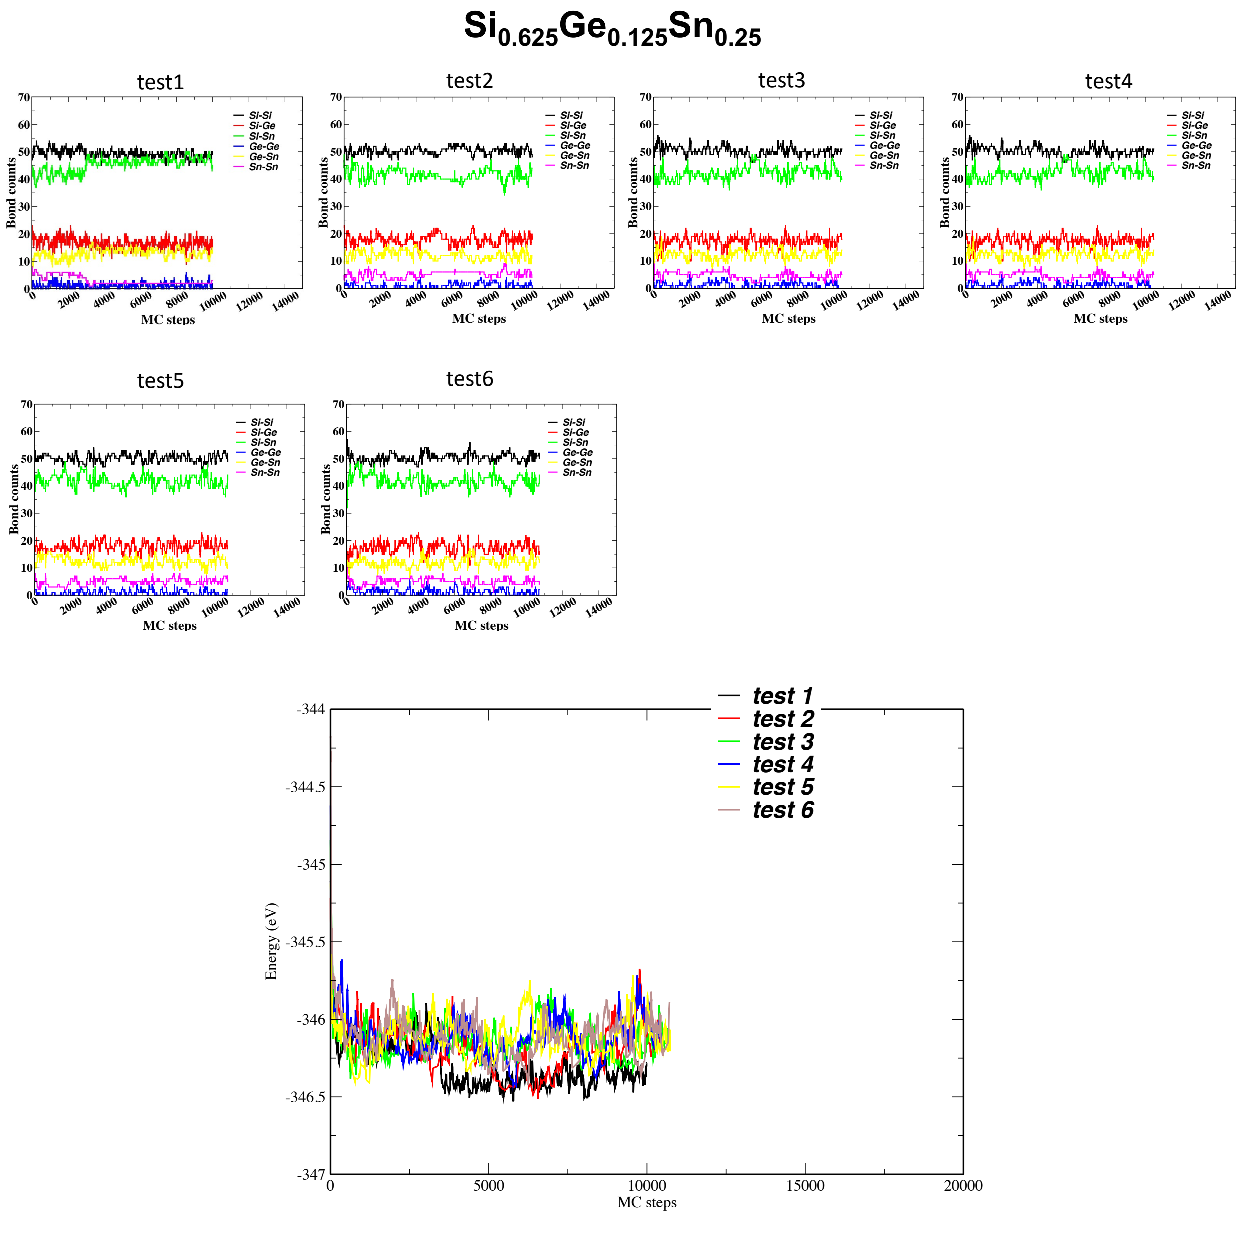


Figure S11: Variation of energy and bonds in MC/DFT sampling for $Si_{0.625}Ge_{0.125}Sn_{0.25}$

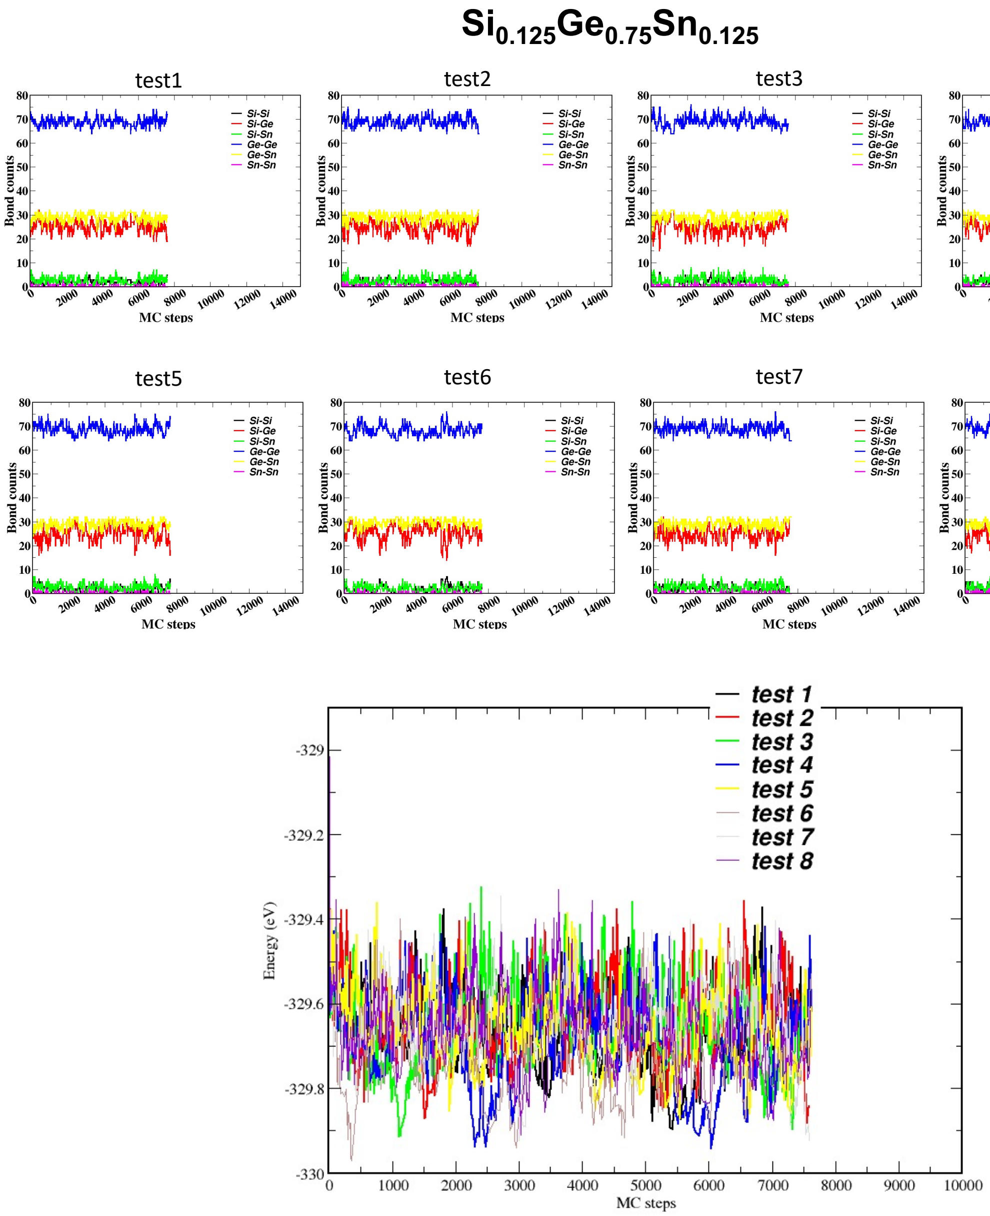


Figure S12: Variation of energy and bonds in MC/DFT sampling for $Si_{0.125}Ge_{0.75}Sn_{0.125}$

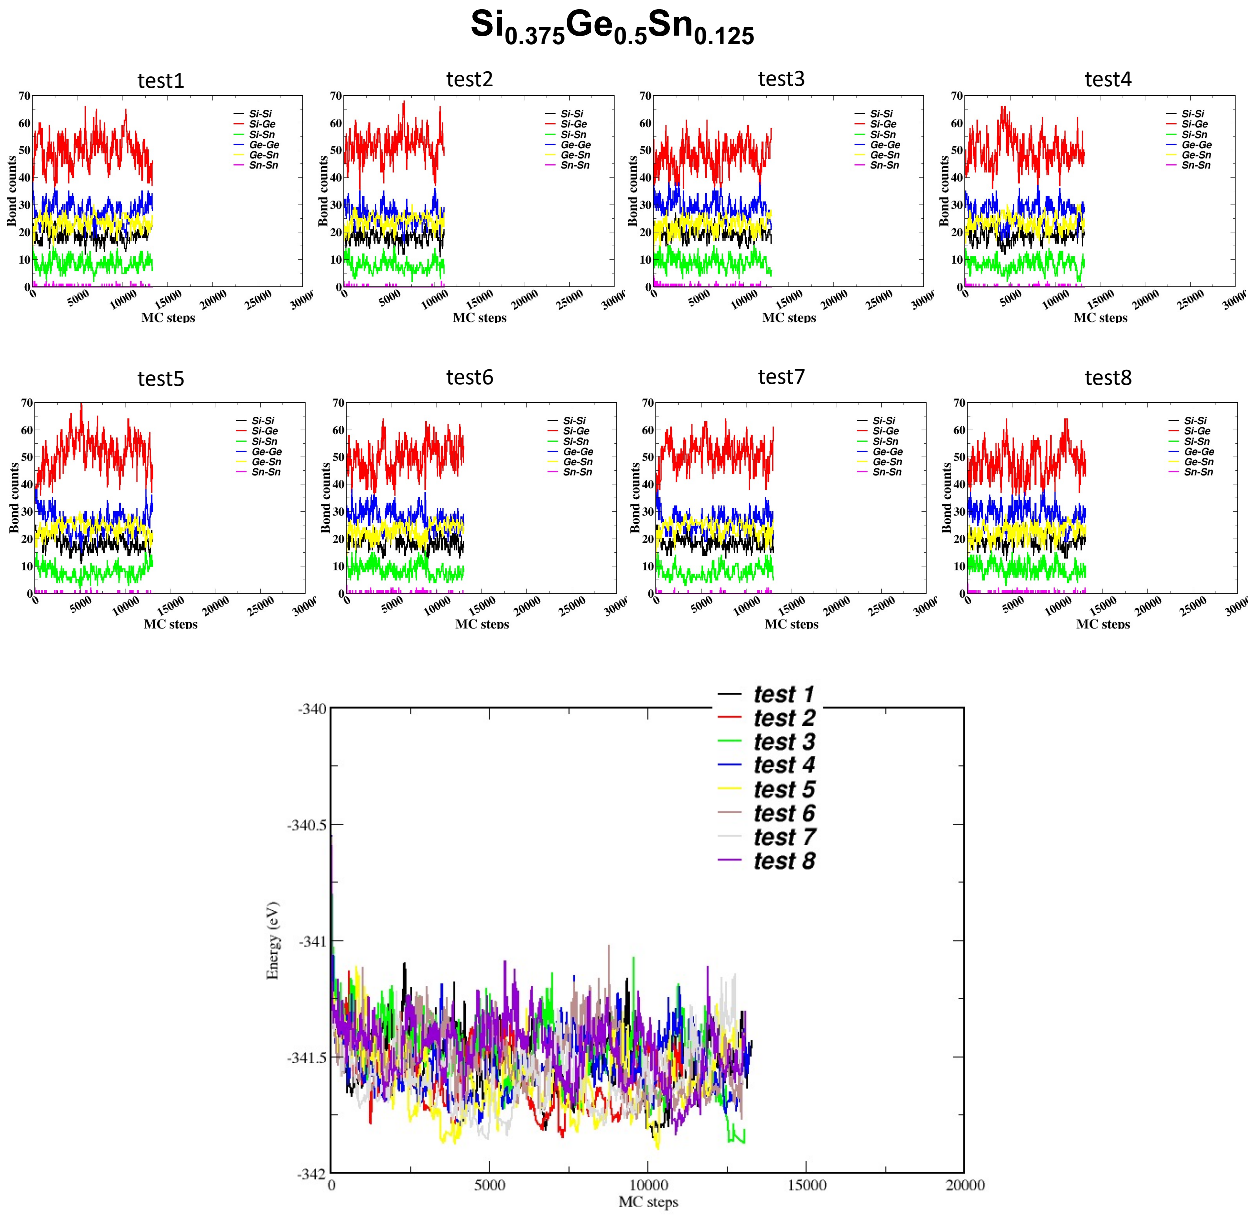


Figure S13: Variation of energy and bonds in MC/DFT sampling for $Si_{0.375}Ge_{0.5}Sn_{0.125}$

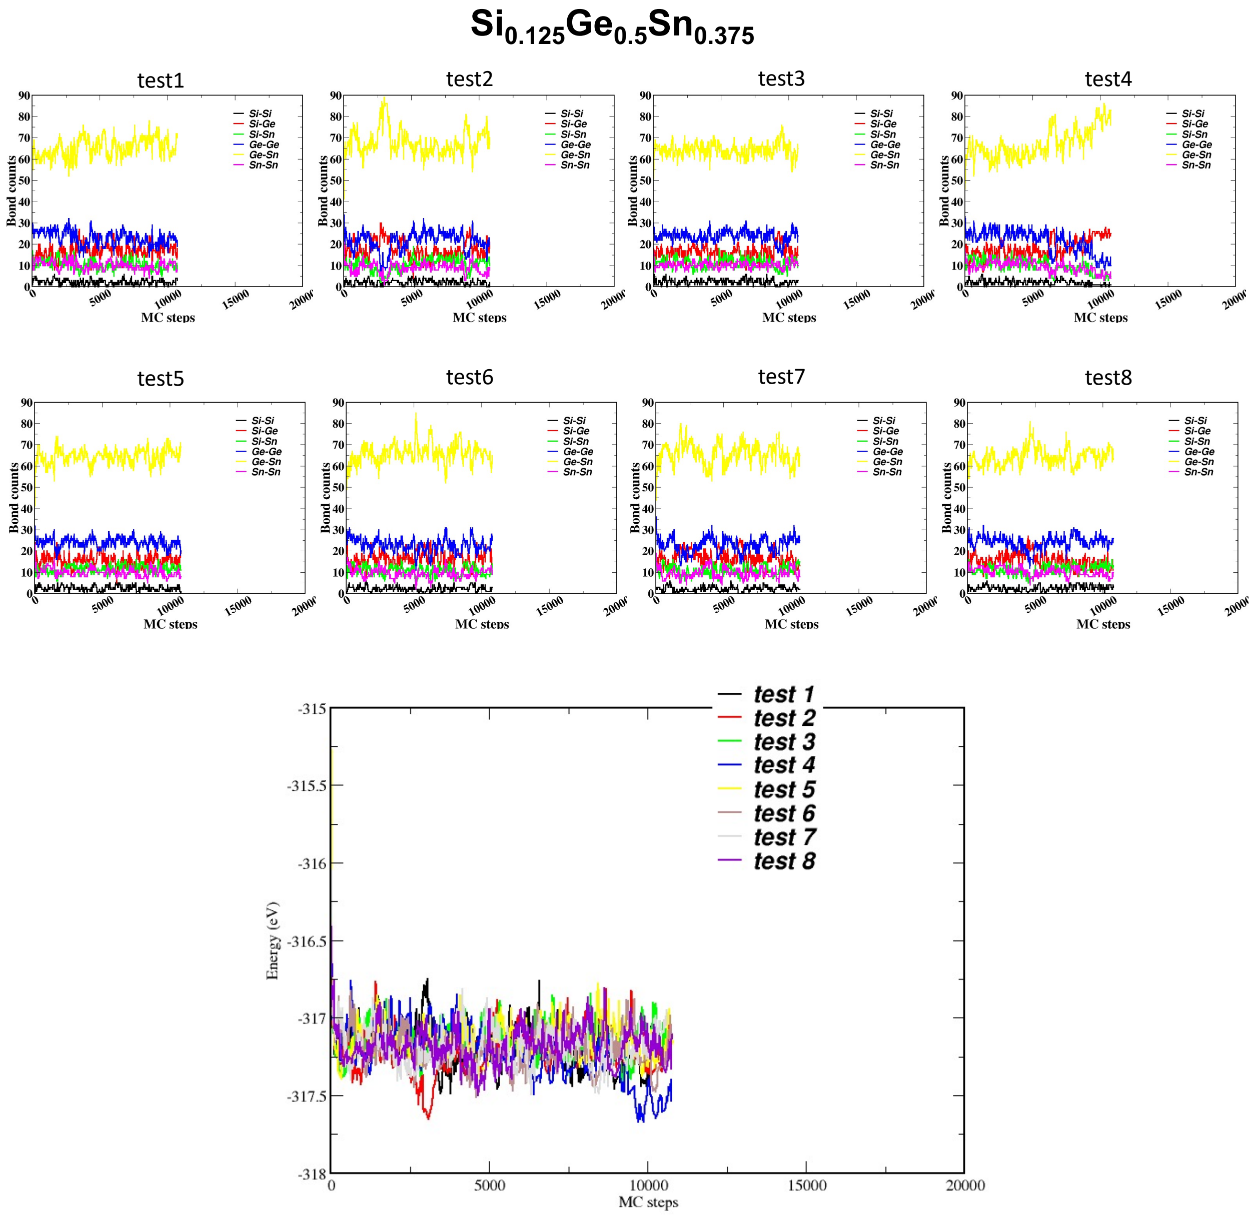


Figure S14: Variation of energy and bonds in MC/DFT sampling for $Si_{0.125}Ge_{0.5}Sn_{0.375}$

Table S1: Vibrational Helmholtz free energy of mixing $\Delta F_{mix}^{vib}$, obtained from random, R-SRO, and E-SRO, for different compositions, showing little difference between R-SRO and E-SRO.

| Composition | $\Delta F_{mix}^{vib}$ (meV/atom) | | |
|---|---|---|---|
| | Random | R-SRO | E-SRO |
| $Si_{0.125}Ge_{0.625}Sn_{0.25}$ | -1.63 | -0.49 | -0.30 |
| $Si_{0.25}Ge_{0.5}Sn_{0.25}$ | -1.05 | -0.02 | 0.13 |

Table S2: Equilibrium lattice constants of SiGeSn, obtained from random, R-SRO, and E-SRO, for different compositions, showing the virtual independence of lattice constant on the degree of ordering.

| Composition | Lattice constants (Å) | | |
|---|---|---|---|
| | Random | R-SRO | E-SRO |
| $Si_{0.125}Ge_{0.625}Sn_{0.25}$ | 5.824 | 5.821 | 5.815 |
| $Si_{0.25}Ge_{0.5}Sn_{0.25}$ | 5.791 | 5.788 | 5.781 |
| $Si_{0.375}Ge_{0.375}Sn_{0.25}$ | 5.759 | 5.755 | 5.749 |

# References

(S1) Moutanabbir, O.; Assali, S.; Gong, X.; O'Reilly, E.; Broderick, C. A.; Marzban, B.; Witzens, J.; Du, W.; Yu, S.-Q.; Chelnokov, A.; Buca, D.; Nam, D. Monolithic infrared silicon photonics: The rise of (Si)GeSn semiconductors. *Applied Physics Letters* **2021**, *118*, 110502.
